# Supplementary material for: Description of seismic sources in underground mines: Dynamic stress fracturing around tunnels and strainbursting
Source: arXiv:2205.07379 ancillary file (2022-05-15)
Supplement: Supplementary file 1 [file IMS-NOTE-HBVERIFICATION-202110-v1.pdf]

# Verification of strain-softening constitutive models

Alex Rigby

October 15, 2021

## 1 Introduction

This report presents verification test results of strain-softening Hoek-Brown (HB) and Mohr-Coulomb (MC) constitutive models, which have been implemented based on the formulation of Refs. [1, 2]. Taking compression as positive, the HB yield function can be written as

$$f(\sigma_1, \sigma_3) = \sigma_3 - \sigma_1 + \sigma_{ci} \left( m_b \frac{\sigma_3}{\sigma_{ci}} + s \right)^a, \quad (1)$$

where  $\sigma_{ci}$  is the uniaxial compressive strength and  $m_b$ ,  $a$ , and  $s$  are the HB constants. Plastic flow is governed by a potential function of the same form with different coefficients:

$$g(\sigma_1, \sigma_3) = \sigma_3 - \sigma_1 + \sigma_{cig} \left( m_{bg} \frac{\sigma_3}{\sigma_{cig}} + s_g \right)^{a_g}. \quad (2)$$

Each of the eight coefficients in Eqs. 1 and 2 are functions of plastic strain  $\epsilon^p$ . In particular, we take them to be functions of deviatoric plastic strain  $\bar{\epsilon}^p = \epsilon_1^p - \epsilon_3^p$ , where  $\epsilon_1^p$  and  $\epsilon_3^p$  are the major and minor eigenvalues of plastic strain, respectively.

The MC yield function can be written as

$$f(\sigma_1, \sigma_3) = k_\phi \sigma_3 - \sigma_1 + \sigma_c, \quad (3)$$

where  $k_\phi = (1 + \sin \phi)/(1 - \sin \phi)$ ,  $\sigma_c = 2c \cos \phi/(1 - \sin \phi)$ ,  $\phi$  is the friction angle, and  $c$  is the cohesion. The potential function can be written as

$$g(\sigma_1, \sigma_3) = k_\psi \sigma_3 - \sigma_1, \quad (4)$$

where  $k_\psi = (1 + \sin \psi)/(1 - \sin \psi)$  and  $\psi$  is the dilation angle. It follows that the MC constitutive model can be implemented as a special case of the HB model with  $\sigma_{ci} = \sigma_c$ ,  $m_b = k_\phi - 1$ ,  $a = 1$ ,  $s = 1$ ,  $m_{bg} = k_\psi - 1$ , and  $a_g = 1$ . The values used for  $\sigma_{cig}$  and  $s_g$  are unimportant as plastic flow depends on the derivative  $\partial g/\partial \sigma_3$ , which is simply  $1 + m_{bg}$  for  $a_g = 1$ .

## 2 Methodology

Each of the cases considered is based on a 10m radius circular tunnel. Simulation is conducted using IMS's Material Point Method implementation, which is based of the formulations of [3, 4]. A common mesh composed of a single layer of tetrahedra produced using TETGEN [5] is used, a reduced-size version of which is shown in Fig. 1. In practice, the square mesh used has a diameter of 1000m and each concentric annulus of tetrahedra is defined by 48 vertices.

Each of the tetrahedra is populated with four particles whose initial stress is set according to a hydrostatic loading. Supposing the tunnel is north-south oriented, fixed displacement conditions are

applied at the top, bottom, east, and west boundaries; fixed normal displacement (roller) conditions are applied at the north and south boundaries.

The simulation of each case is performed in two stages: Initially, the simulation is run to quasi-static equilibrium (using damping as described in [6, 7]) under the restriction that the material (rockmass) behaves elastically. In the second stage, failure is permitted according to the HB or MC criteria described in Section 1, and simulation continues until the system returns to equilibrium.

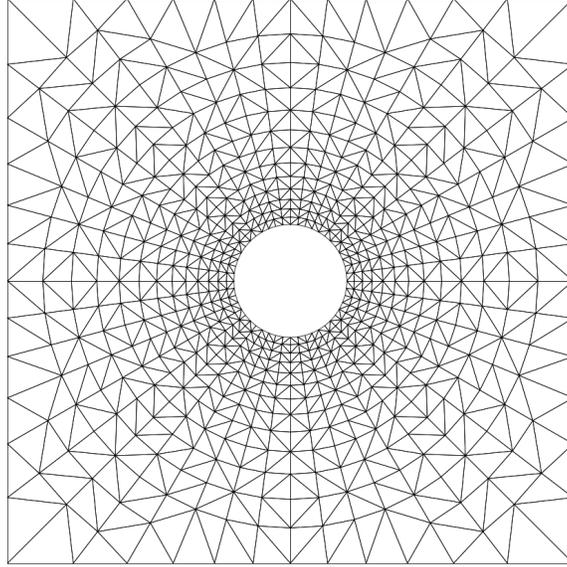

Figure 1: Simplified example of the employed mesh geometry.

### 3 Results

#### 3.1 Case 1 – perfectly plastic HB

In the first case considered, the HB rockmass behaves perfectly plastically after failure, meaning that the yield and potential surface parameters remain constant. These parameters are listed and shown graphically in Fig. 2. The applied load pressure in this case is 150 MPa.

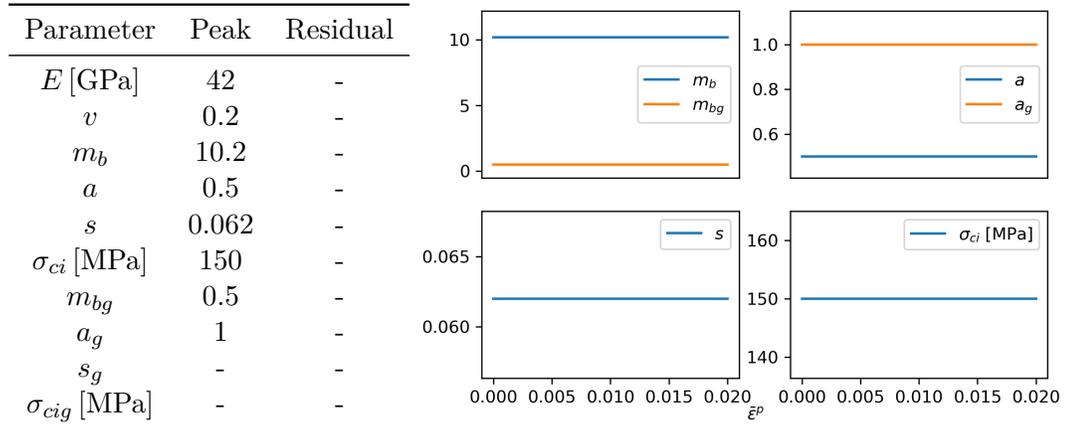

Figure 2: Case 1 material parameters.

Following convergence of the simulation, values of radial displacement  $u_r$ , radial stress  $\sigma_r$ , and tangential stress  $\sigma_\theta$  are determined by averaging over the particles belonging to each annulus of the mesh. As shown in Fig. 3, these values are then compared to the analytical solutions published in Ref. [8]. It can be seen that there is good agreement between the analytical and modelled values.

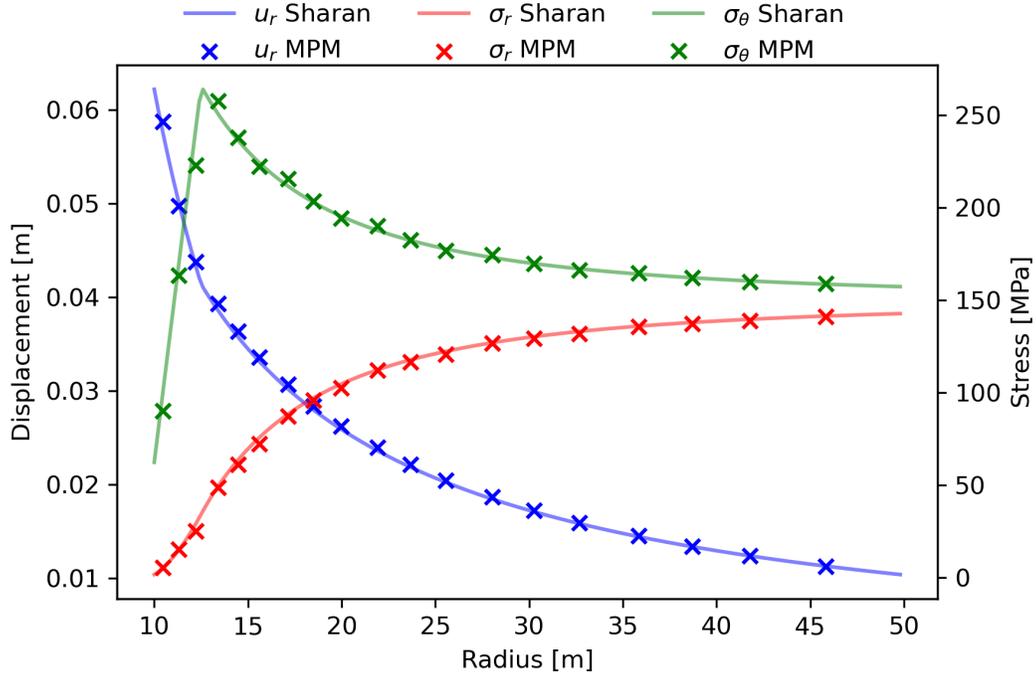

Figure 3: Case 1 results.

### 3.2 Case 2 – brittle plastic HB

In the second case considered, the HB rockmass is brittle, meaning that the yield and potential surface parameters (as shown in Fig. 4) drop to residual values immediately following initial failure. The applied load pressure is 75 MPa.

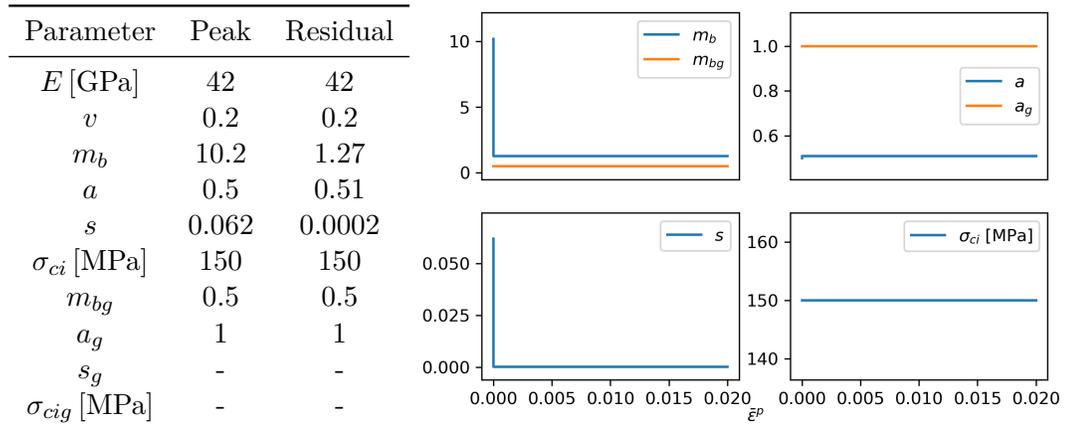

Figure 4: Case 2 material parameters.

Again, the obtained solution is compared to that of Ref. [8]. It can be seen that there is good agreement between the analytical and modelled values.

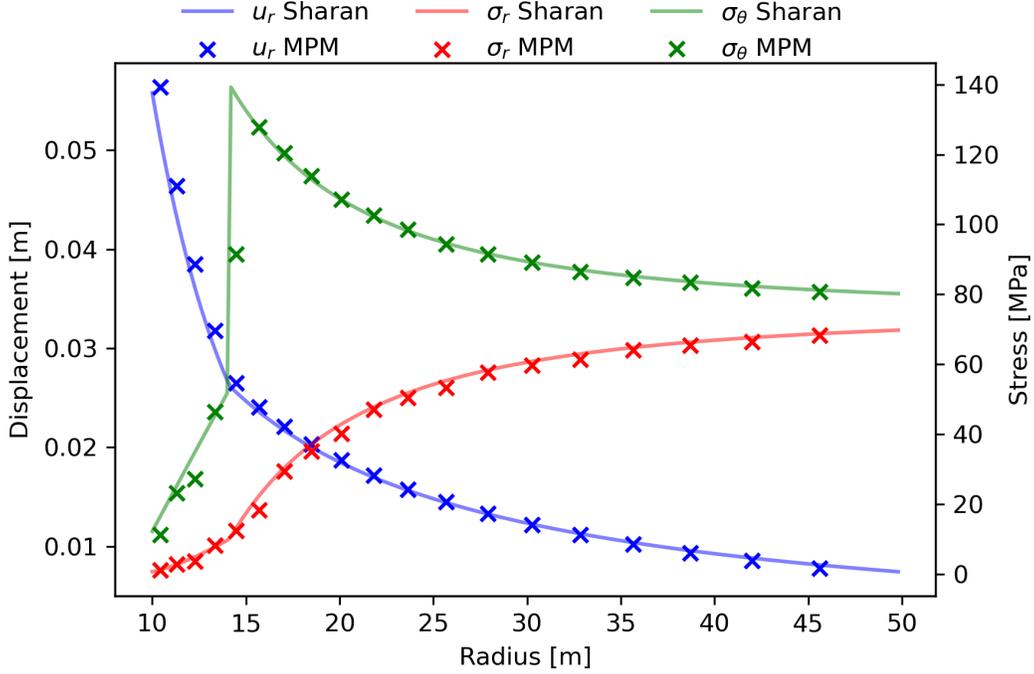

Figure 5: Case 2 results.

### 3.3 Case 3 – strain-softening HB

In the third case considered, the HB rockmass softens after initial failure. In particular, as shown in Fig. 6, the yield and potential surface parameters change linearly with  $\bar{\epsilon}^p$  until a value of  $\bar{\epsilon}^p = 0.01$ , after which they remain at constant residual values. The load pressure is 15 MPa.

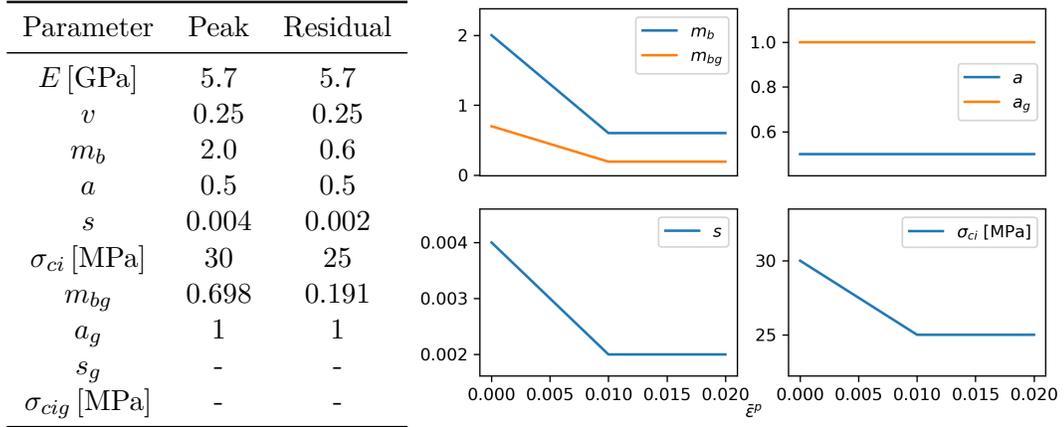

Figure 6: Case 3 material parameters.

In this case, the model solution is compared in Fig. 7 to that obtained from the finite-difference method approach outlined in Ref. [9]. Again, a good agreement is observed.

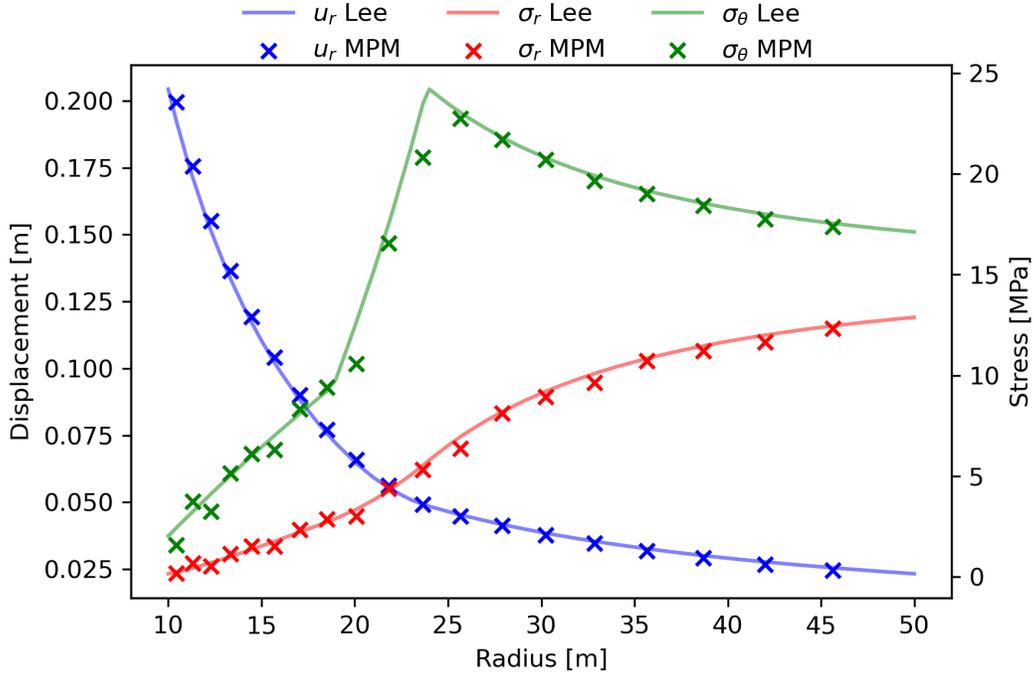

Figure 7: Case 3 results.

### 3.4 Case 4 – strain-softening MC

The final case considered is that of a strain-softening MC rockmass. The relevant parameters are given in Fig. 8. Again, these parameters change linearly after initial failure, this time up to a value of  $\bar{\epsilon}^p = 0.008$ . The load pressure is 20 MPa.

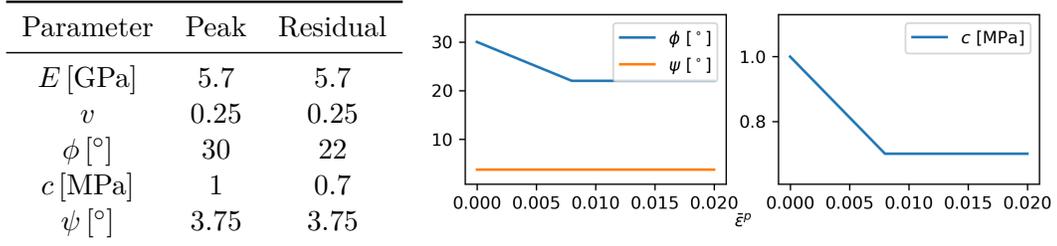

Figure 8: Case 4 material parameters.

As with HB case, the model solution is compared that of Ref. [8]. This is shown in Fig. 9, where a good agreement can be observed.

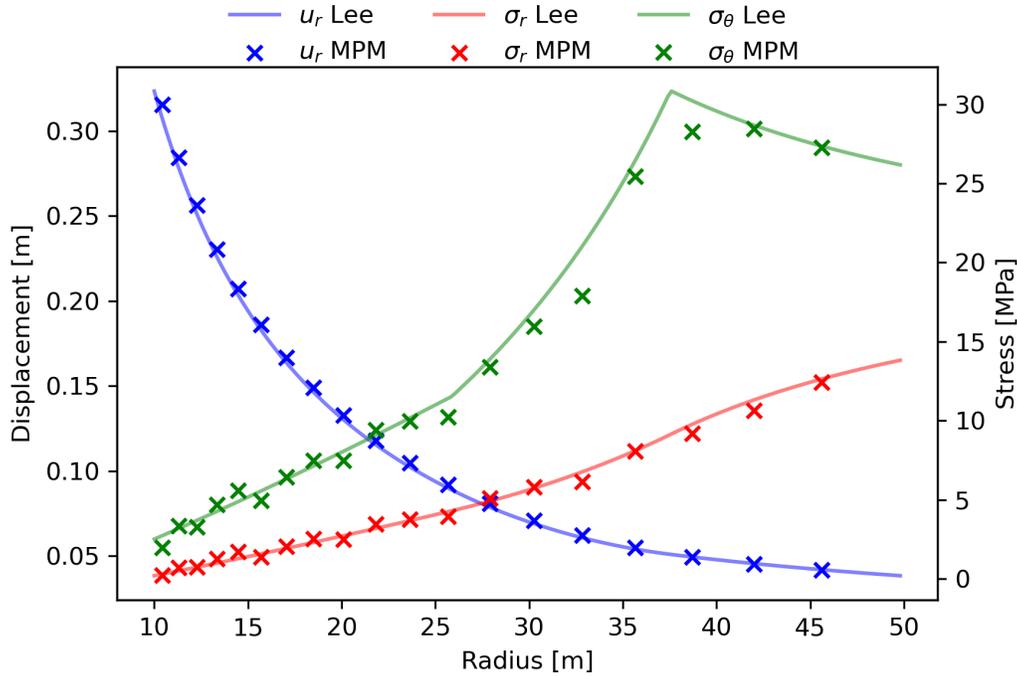

Figure 9: Case 3 results.

## References

- [1] E. S. Sørensen, J Clausen, and L. Damkilde, “Finite element implementation of the Hoek–Brown material model with general strain softening behavior,” *International Journal of Rock Mechanics and Mining Sciences*, vol. 78, pp. 163–174, 2015.
- [2] E. Sørensen, “Numerical simulation of non-linear phenomena in geotechnical engineering,” English, PhD supervisor: Prof. Lars Damkilde, Aalborg University Assistant PhD supervisor: Assoc. Prof. Johan Clausen, Aalborg University, PhD thesis, 2016. DOI: [10.5278/vbn.phd.engsci.00108](https://doi.org/10.5278/vbn.phd.engsci.00108).
- [3] I. Jassim, “Formulation of a dynamic material point method (mpm) for geomechanical problems,” PhD thesis, Institute of Geotechnical Engineering, University of Stuttgart, 2013.
- [4] J. A. Nairn, “Material point method calculations with explicit cracks,” *Computer Modeling in Engineering and Sciences*, vol. 4, no. 6, pp. 649–664, 2003.
- [5] H. Si, “TetGen, a Delaunay-based quality tetrahedral mesh generator,” *ACM Transactions on Mathematical Software (TOMS)*, vol. 41, no. 2, pp. 1–36, 2015.
- [6] B. Wang, P. J. Vardon, M. A. Hicks, and Z. Chen, “Development of an implicit material point method for geotechnical applications,” *Computers and Geotechnics*, vol. 71, pp. 159–167, 2016.
- [7] Itasca Consulting Group, *FLAC3D: Fast Lagrangian Analysis of Continua in 3 Dimensions. Theory and background*, 4.0, 2009.
- [8] S. K. Sharan, “Analytical solutions for stresses and displacements around a circular opening in a generalized Hoek-Brown rock,” *International journal of rock mechanics and mining sciences (1997)*, vol. 45, no. 1, pp. 78–85, 2008.
- [9] Y.-K. Lee and S Pietruszczak, “A new numerical procedure for elasto-plastic analysis of a circular opening excavated in a strain-softening rock mass,” *Tunnelling and Underground Space Technology*, vol. 23, no. 5, pp. 588–599, 2008.
