# Supplementary material for: Description of seismic sources in underground mines: Dynamic stress fracturing around tunnels and strainbursting
Source: arXiv:2205.07379 ancillary file (2022-05-15)
Supplement: Supplementary file 2 [file IMS-NOTE-MPMVERIFICATION-202009-v1.pdf]

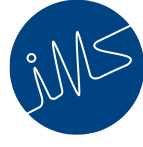

institute  
of mine  
seismology

## Verification of IMS MPM implementation

Alex Rigby, Dmitriy Malovichko, Gys Basson

23rd April 2021

IMS-NOTE-MPMVERIFICATION-202009-IMS-v1

### Contents

|          |                                                     |           |
|----------|-----------------------------------------------------|-----------|
| <b>1</b> | <b>Introduction</b>                                 | <b>1</b>  |
| <b>2</b> | <b>Elastostatic, 2D elliptical cavity [1]</b>       | <b>2</b>  |
| 2.1      | Case 1 - $a = 3$ m, $b = 2.5$ m, $\beta = 90^\circ$ | 2         |
| 2.2      | Case 2 - $a = 3$ m, $b = 2.5$ m, $\beta = 30^\circ$ | 3         |
| 2.3      | Case 3 - $a = 3$ m, $b = 0.5$ m, $\beta = 30^\circ$ | 3         |
| <b>3</b> | <b>Mohr-Coulomb, cylindrical cavity [2]</b>         | <b>10</b> |
| 3.1      | Case 4 - $P_i = 0$ MPa                              | 10        |
| 3.2      | Case 5 - $P_i = 5$ MPa                              | 10        |
| <b>4</b> | <b>Hoek-Brown, cylindrical cavity [3]</b>           | <b>15</b> |
| 4.1      | Case 6 - non-associated                             | 15        |
| 4.2      | Case 7 - associated                                 | 15        |

### 1 Introduction

The objective of this document is to test the validity of the approximate solutions of IMS's MPM (material point method) modelling software by comparison to known analytical solutions across a number of cases. In particular, we compare the Cartesian components of stress  $\sigma$  and induced displacement  $\mathbf{u}$  (total displacement minus cavity-free displacement) in the region of different cavities.

MPM yields approximate solutions  $\tilde{f}(\mathbf{x}_i)$  at a discrete set of points  $\mathbf{x}_i$ . We quantify the accuracy of these solutions within a distance  $d$  of the cavity  $C$  by considering the misfit to the analytical values  $f(\mathbf{x}_i)$ ,

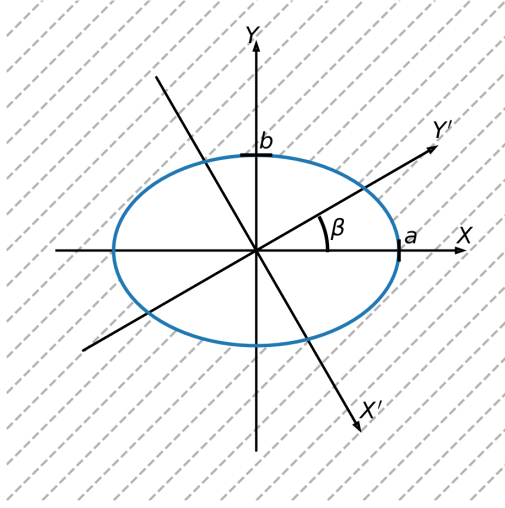

(a) Elliptical cavity geometry.

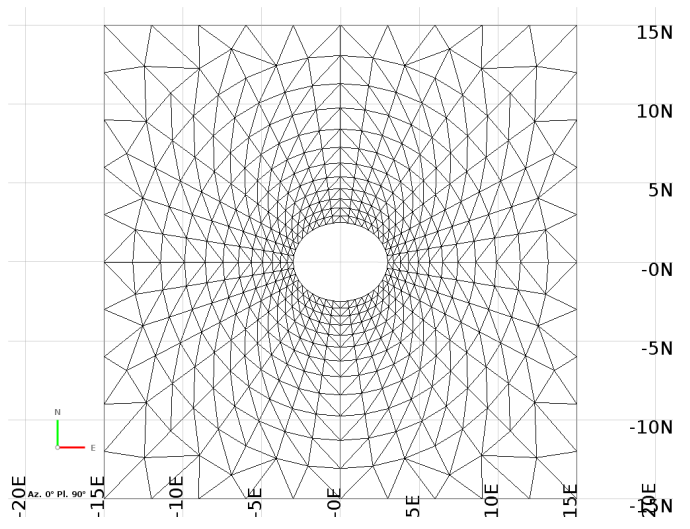

(b) Top-down view of a simplified version of the tetrahedral grid used in MPM simulation.

Figure 1

which we calculate as

$$M(d) = \frac{\sum_{\mathbf{x}_i: \text{dist}(\mathbf{x}_i, C) < d} |\tilde{f}(\mathbf{x}_i) - f(\mathbf{x}_i)|}{\sum_{\mathbf{x}_i: \text{dist}(\mathbf{x}_i, C) < d} |f(\mathbf{x}_i)|}. \quad (1)$$

## 2 Elastostatic, 2D elliptical cavity [1]

Ref. [1] provides analytical solutions for stress and displacement in an elastic medium around a 2D elliptical cavity that is biaxially loaded. The geometry of the system is shown in Fig. 1a. The ellipse has semi-major and semi-minor axes  $a$  and  $b$ , respectively. The major loading axis  $Y'$  is at an angle  $\beta$  to the major axis of the ellipse, which lies on the  $X$ -axis.

For all cases considered in this section, the elastic medium is taken to have Lamé parameters  $\mu = 30$  GPa and  $\lambda = 30$  GPa, which corresponds to a Young's modulus of  $E = 75$  GPa and Poisson's ratio of  $\nu = 0.25$ . Loading, which is taken to be compression positive, is 50 MPa and 20 MPa along the  $Y'$ - and  $X'$ - axes, respectively. Plane strain is assumed.

For the MPM simulations, a thin plate meshed with a single symmetrical layer of tetrahedra is used. A simplified top-down view of the mesh geometry is shown in Fig. 1b. In practice, 200 vertices are used around the cavity's circumference, and the plates have a diameter of  $D = 200 \text{ m} \gg a$ . Each cell (tetrahedron) is populated with eight particles with an initial stress equal to the in situ stress considered. Fixed displacement conditions are employed at the  $X$  and  $Y$  boundaries, while fixed normal component conditions (rollers) are used at the  $Z$  boundaries.

### 2.1 Case 1 - $a = 3 \text{ m}$ , $b = 2.5 \text{ m}$ , $\beta = 90^\circ$

In the first case considered, the cavity is near circular, with  $a = 3 \text{ m}$  and  $b = 2.5 \text{ m}$ . The loading angle of  $\beta = 90^\circ$  means that the major loading axis is aligned with the minor axis of the ellipse. This gives an in situ stress tensor of

$$\sigma_s = \begin{pmatrix} 20 & 0 & 0 \\ 0 & 50 & 0 \\ 0 & 0 & 17.5 \end{pmatrix} \text{ MPa}.$$

Figure 2 shows contour plots of the analytical and MPM solutions. As noted in Sec. 1, we give the Cartesian components of stress and induced displacement. Figure 3 shows the misfits as defined in Eq.

Table 1: Case 1 to 7 percentage misfits within 15 m of cavity.

| Case | $\sigma_{xx}$ | $\sigma_{yy}$ | $\sigma_{xy}$ | $u_x$ | $u_y$ |
|------|---------------|---------------|---------------|-------|-------|
| 1    | 1.37          | 0.94          | 3.61          | 3.22  | 1.73  |
| 2    | 1.09          | 1.09          | 1.45          | 1.93  | 2.31  |
| 3    | 1.06          | 1.71          | 2.22          | 4.66  | 2.96  |
| 4    | 1.65          | 1.64          | 3.55          | 2.25  | 2.03  |
| 5    | 0.99          | 0.97          | 2.50          | 2.97  | 2.72  |
| 6    | 1.50          | 1.52          | 4.26          | 4.60  | 4.04  |
| 7    | 1.72          | 1.81          | 5.06          | 4.96  | 4.63  |

(1) for up to a distance of 15 m from the cavity. The misfits at 15 m are also given in Table 1 along with those for all other cases considered in this document. Figure 4 compares stress and displacement values in a slice at  $45^\circ$  to the  $X$ -axis (measured anticlockwise). MPM values given are averages obtained by binning the data within  $5^\circ$  of  $45^\circ$  according to distance from the cavity.

## 2.2 Case 2 - $a = 3$ m, $b = 2.5$ m, $\beta = 30^\circ$

In the second case considered, the geometry of the ellipse is unchanged from Case 1, but the major loading axis is now at an angle of  $30^\circ$  from the major axis of the ellipse. This gives an in situ stress tensor of

$$\sigma_s = \begin{pmatrix} 42.5 & 13 & 0 \\ 13 & 27.5 & 0 \\ 0 & 0 & 17.5 \end{pmatrix} \text{ MPa.}$$

Contour plots comparing the solutions are given in Fig. 5, misfits are given in Fig. 6, and values along a slice at  $45^\circ$  are shown in Fig. 7.

## 2.3 Case 3 - $a = 3$ m, $b = 0.5$ m, $\beta = 30^\circ$

In the final elliptical-cavity case considered, the loading is unchanged from Case 2, but the semi-minor axis of the ellipse is reduced to  $b = 0.5$  m. Contour plots comparing the solutions are given in Fig. 8, and misfits are given in Fig. 9, and values along a slice at  $45^\circ$  are shown in Fig. 10.

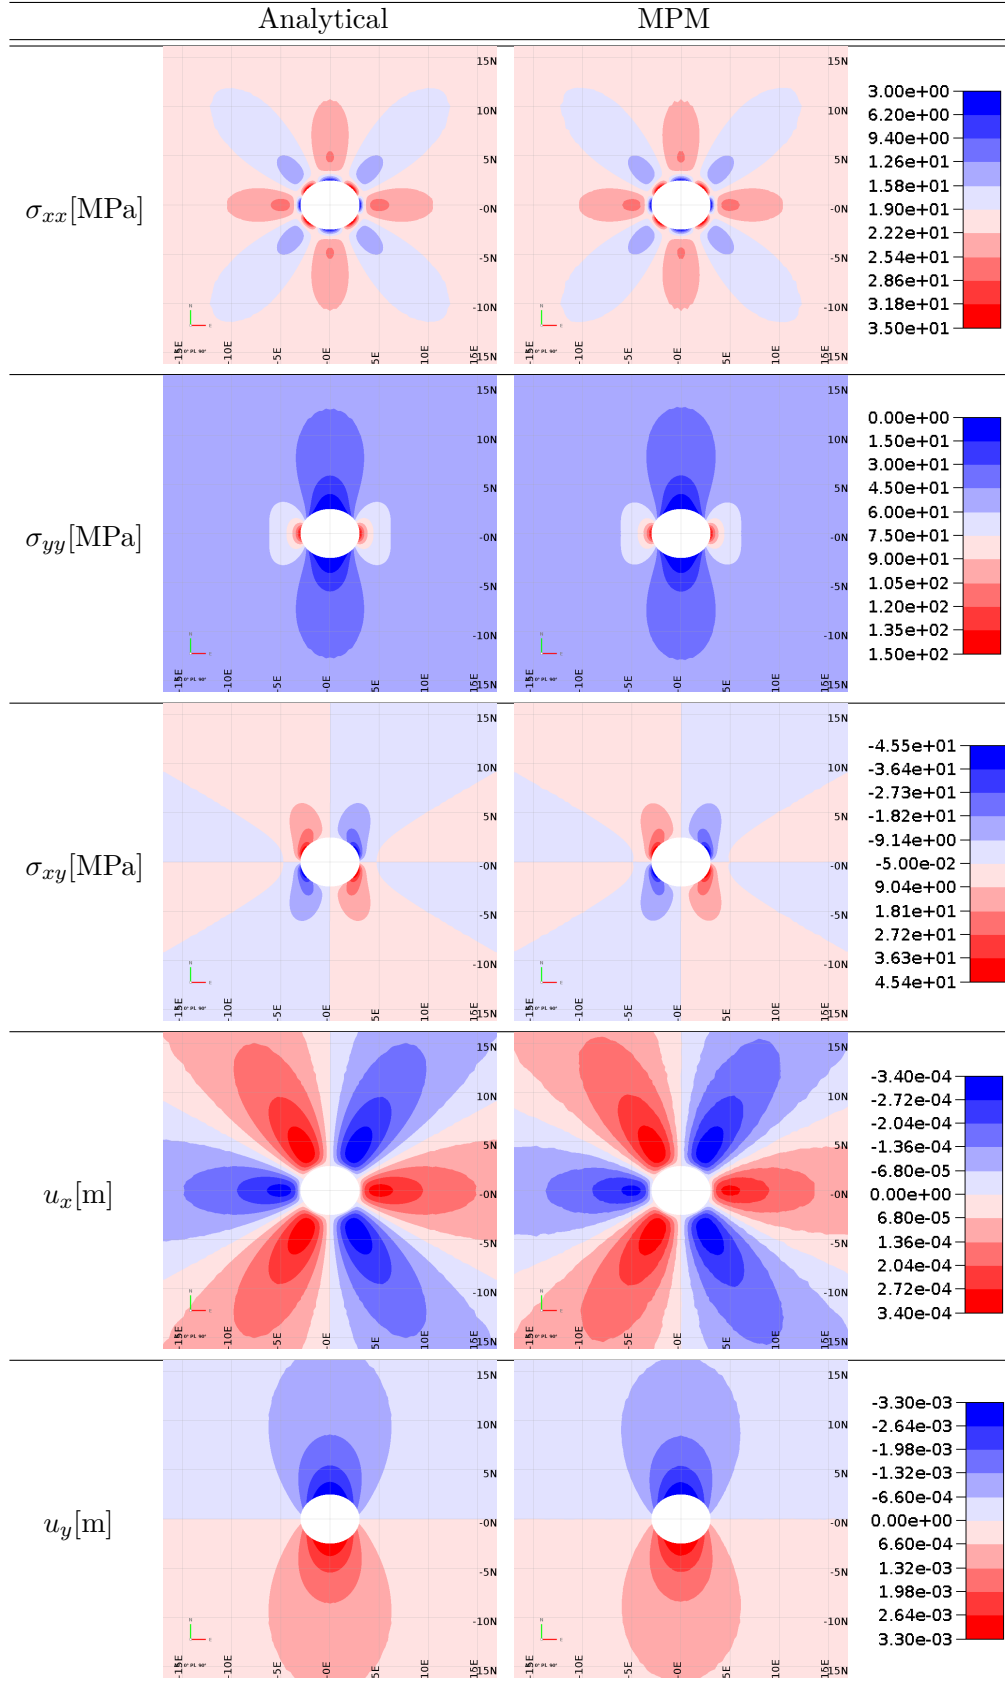

Figure 2: Case 1 stresses and displacements.

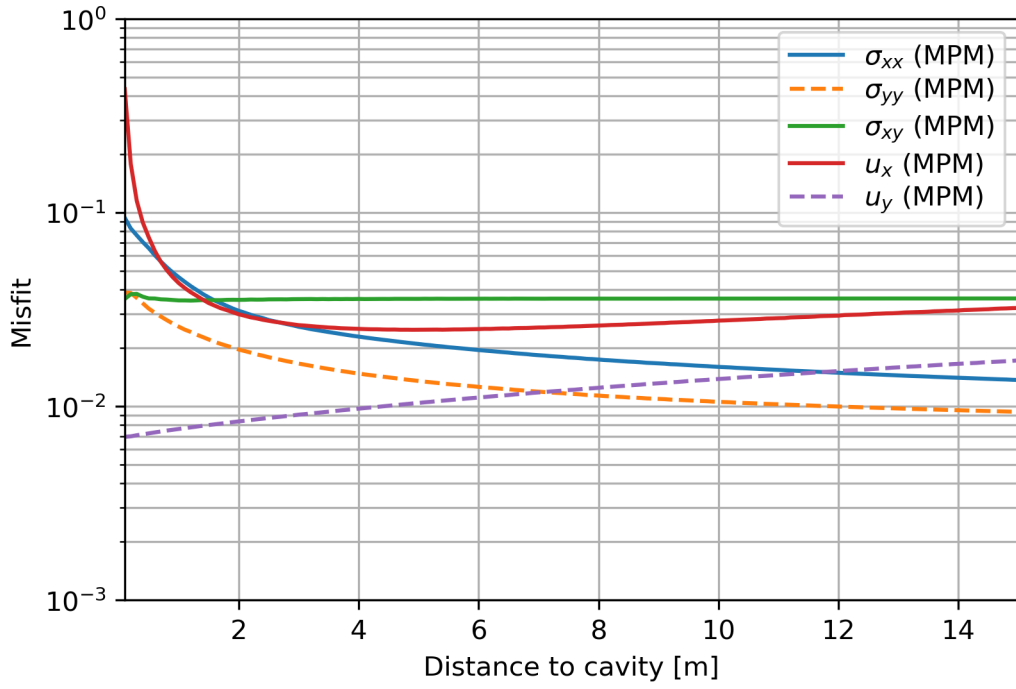

Figure 3: Case 1 misfits.

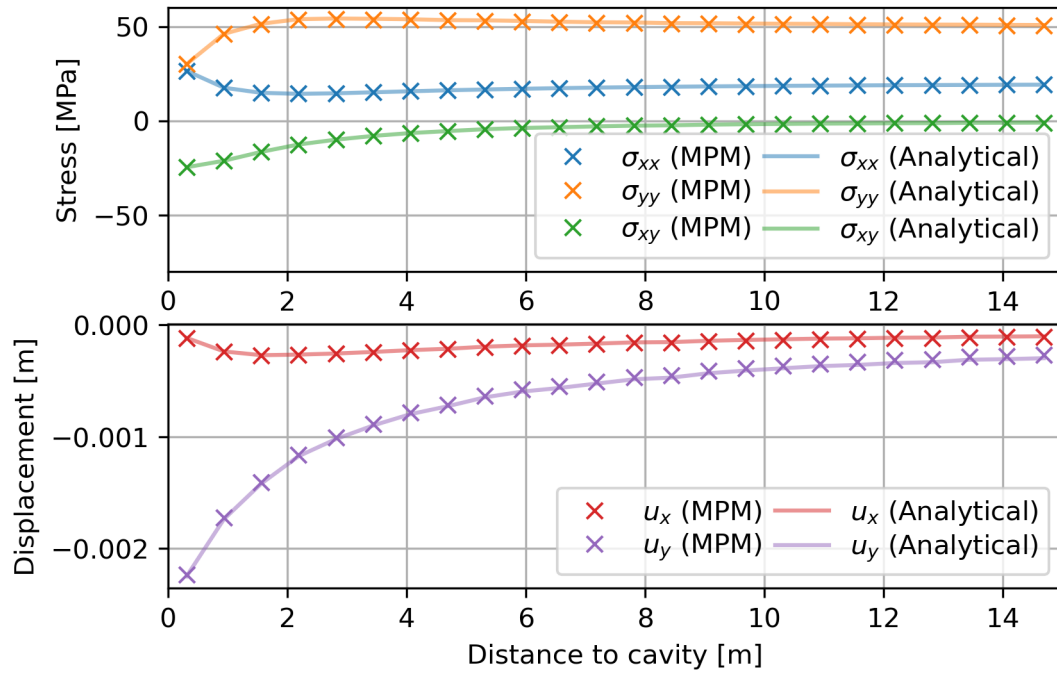

Figure 4: Case 1 stresses and displacements in a slice at  $45^\circ$  to the  $X$ -axis.

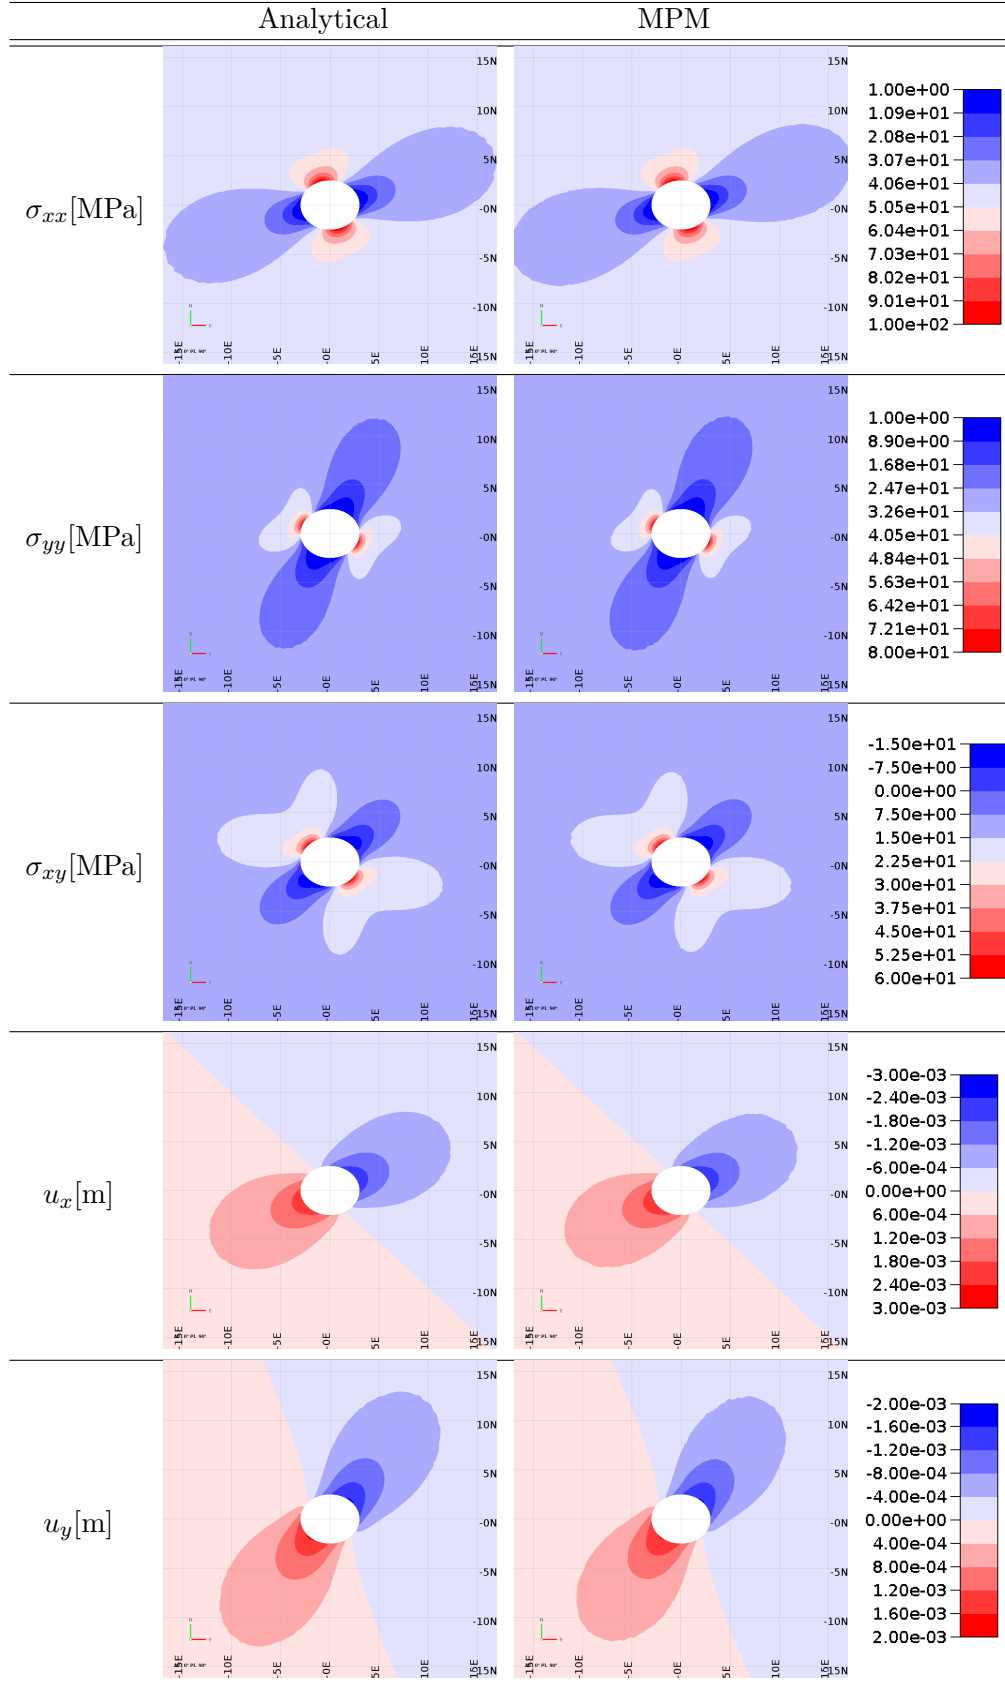

Figure 5: Case 2 stresses and displacements.

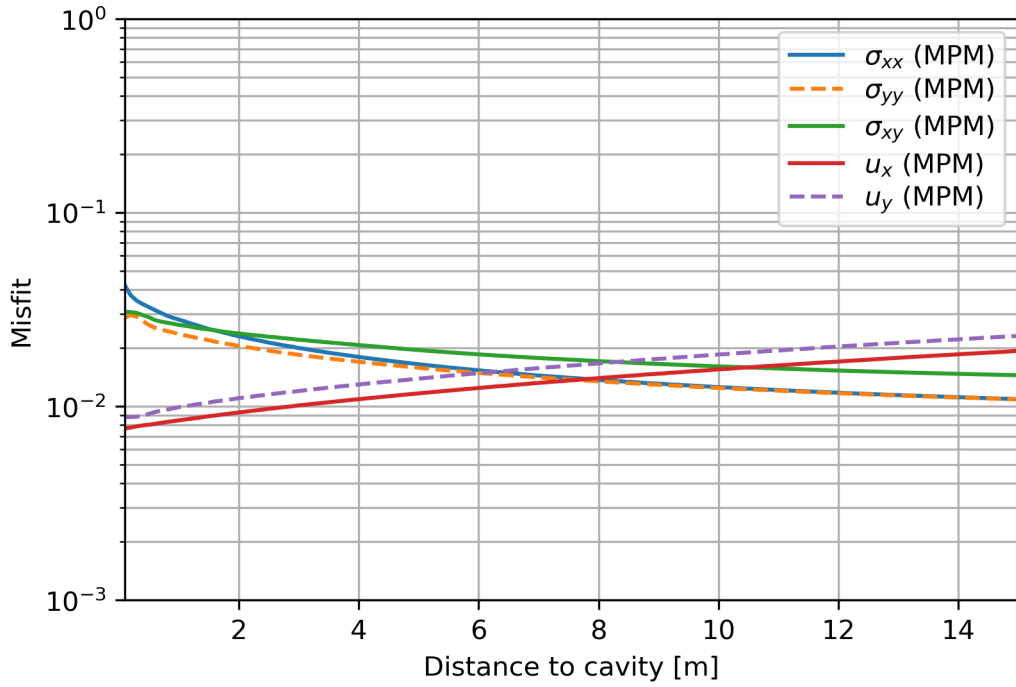

Figure 6: Case 2 misfits.

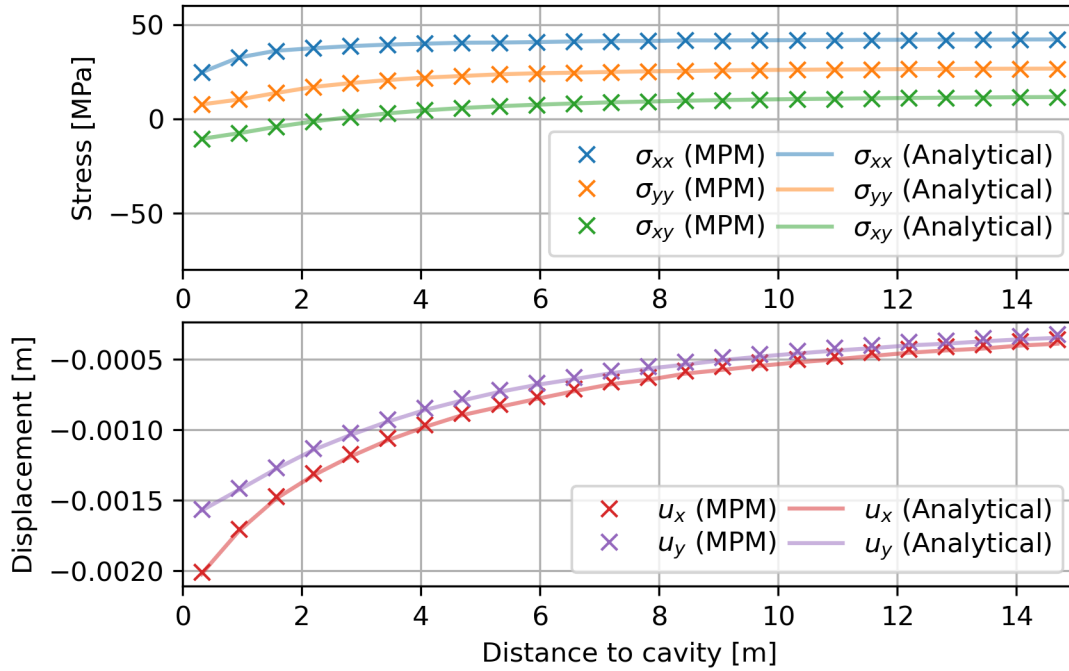

Figure 7: Case 2 stresses and displacements in a slice at  $45^\circ$  to the X-axis.

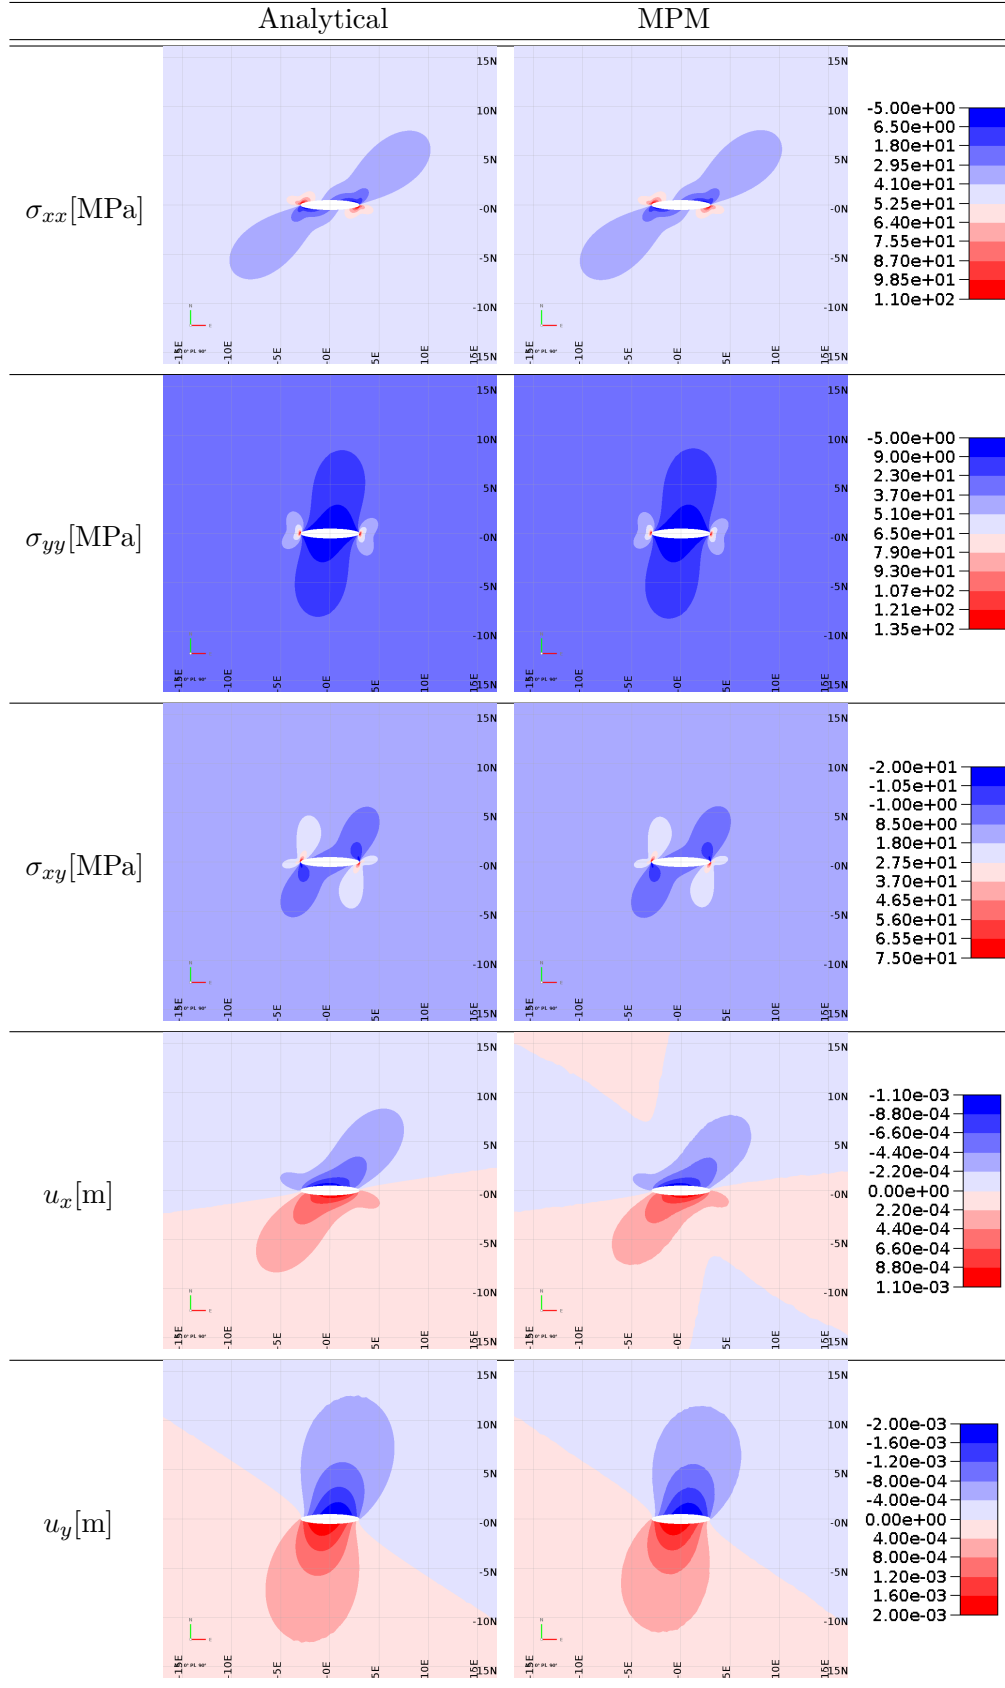

Figure 8: Case 3 stresses and displacements.

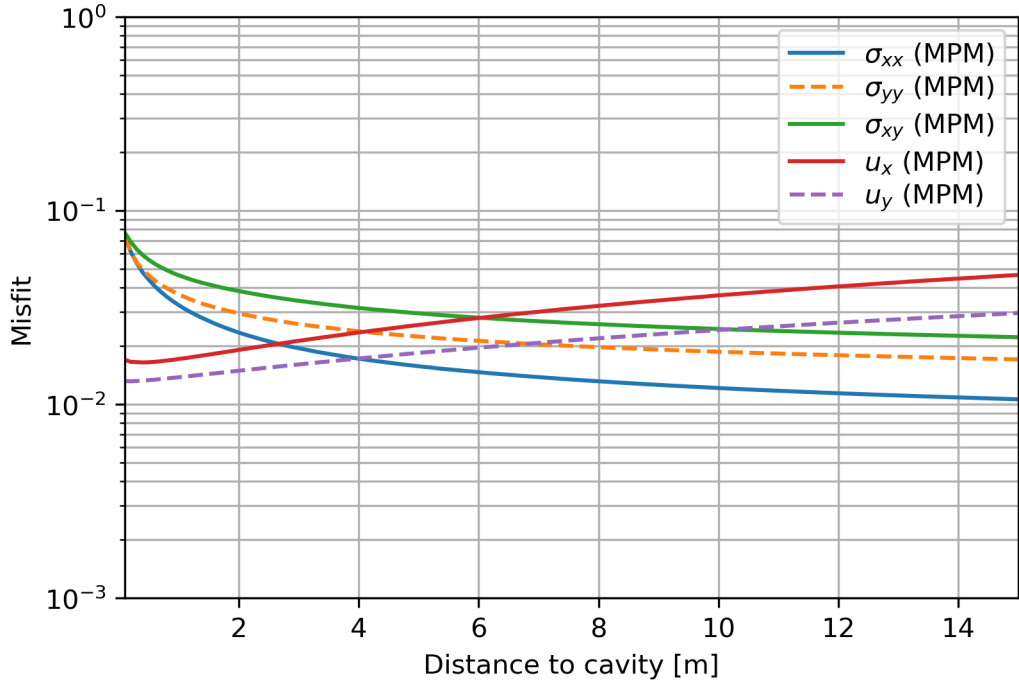

Figure 9: Case 3 misfits.

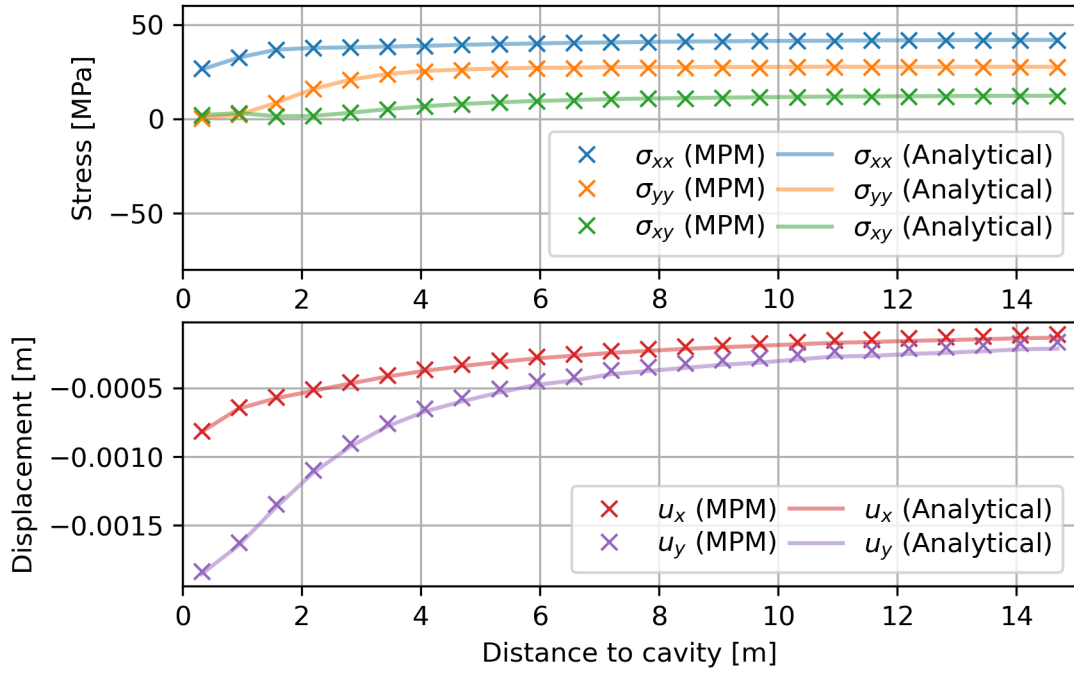

Figure 10: Case 3 stresses and displacements in a slice at  $45^\circ$  to the X-axis.

### 3 Mohr-Coulomb, cylindrical cavity [2]

Ref. [2] provides analytical solutions for stress and displacement in a Mohr-Coulomb material around a cylindrical cavity of infinite length that is isotropically loaded and supported by an internal pressure  $P_i$ . We take this cavity to be oriented along the  $Z$ -axis.

For both cases considered in this section, we take the cylinder's radius to be  $a = 3$  m. The surrounding material has a shear modulus of  $G = 2.8$  GPa, bulk modulus of  $K = 3.9$  GPa ( $E = 67.8$  GPa,  $\nu = 0.210$ ), cohesion of 3.45 MPa, friction angle of  $\phi = 30^\circ$ , and a dilation angle of  $\psi = 0^\circ$ . The isotropic loading is taken to be 30 MPa.

The MPM setup differs in a few ways to that described in Sec. 2: the number of point around the cavities circumference is reduced to 100, fixed normal displacement conditions are used at all boundaries, each cell contains a single particle, and the supporting pressure is implemented by meshing the cavity itself and populating it with low-density elastic particles with fixed isotropic stress defined by  $P_i$ .

#### 3.1 Case 4 - $P_i = 0$ MPa

In the first case considered, the internal pressure is set to zero. Contour plots comparing the solutions are given in Fig. 11. Misfits are given in Fig. 12.

Given the radial symmetry of the geometry in this case, we also show a comparison between the radial stress  $\sigma_r$ , tangential stress  $\sigma_t$ , and radial displacement  $u_r$  (positive away from the cavity) between the MPM and analytical solutions in Fig. 13. The MPM values given are averages obtained by binning the data according to distance from the cavity.

#### 3.2 Case 5 - $P_i = 5$ MPa

In the second case considered, the supporting pressure is set to 5 MPa. Contour plots comparing the solutions are given in Fig. 14, misfits are given in Fig. 15, and radial plots are given in Fig. 16.

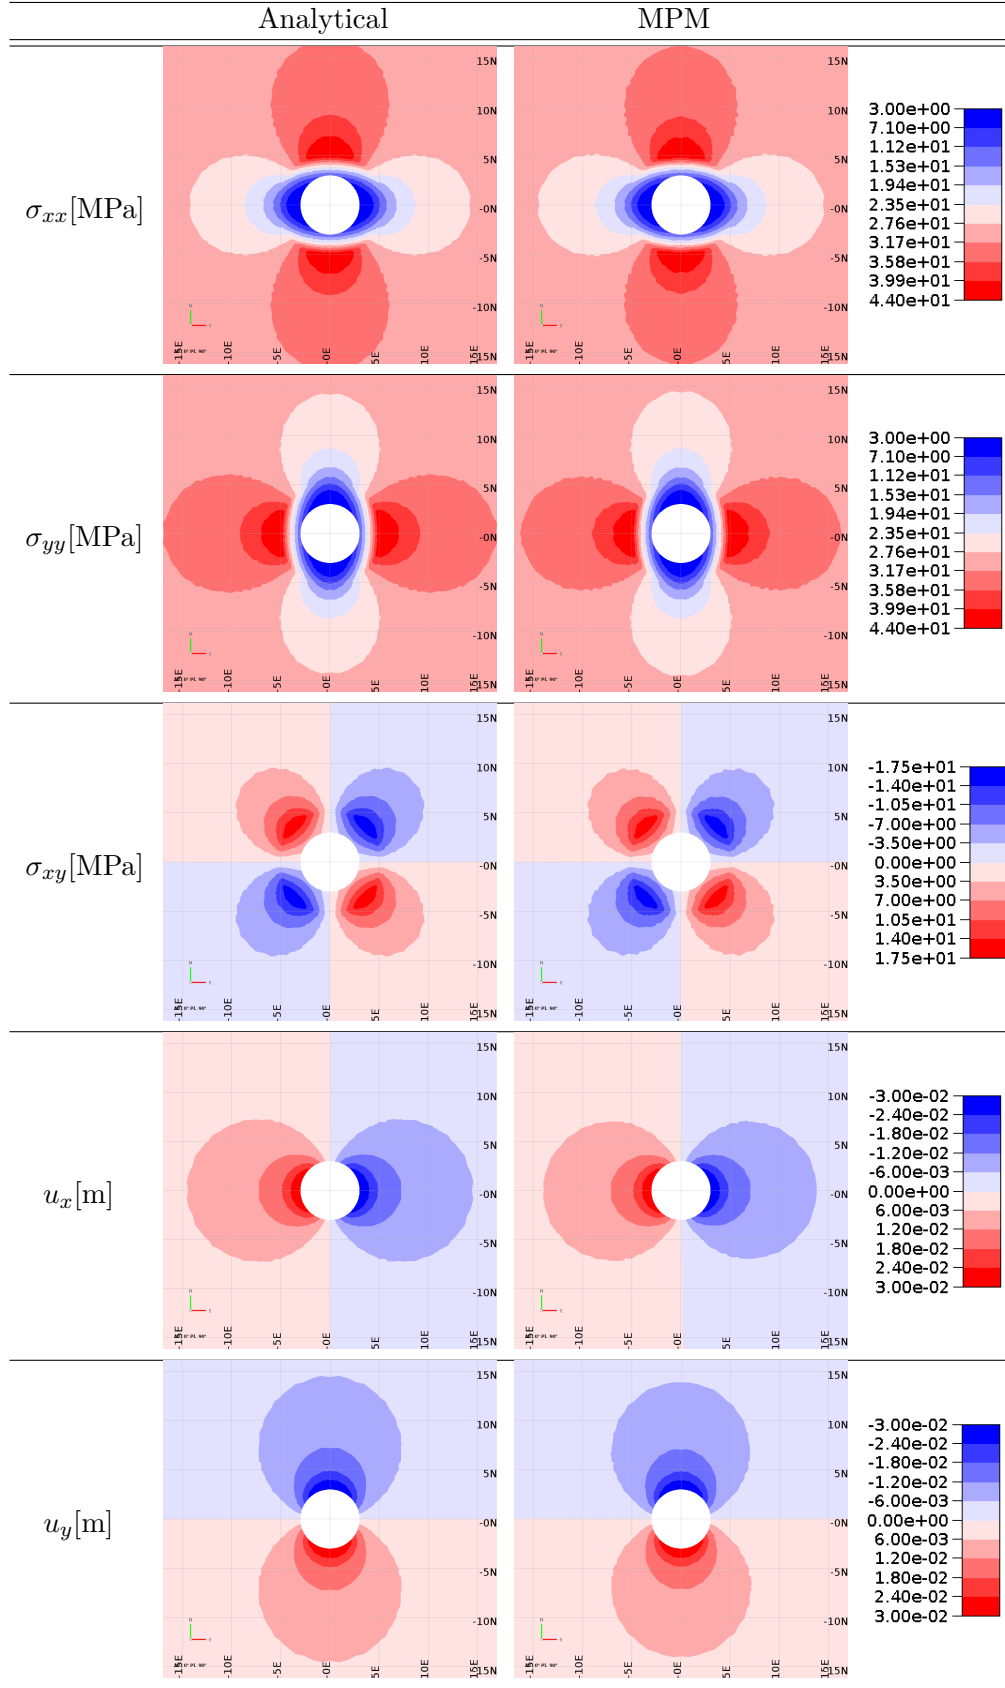

Figure 11: Case 4 stresses and displacements.

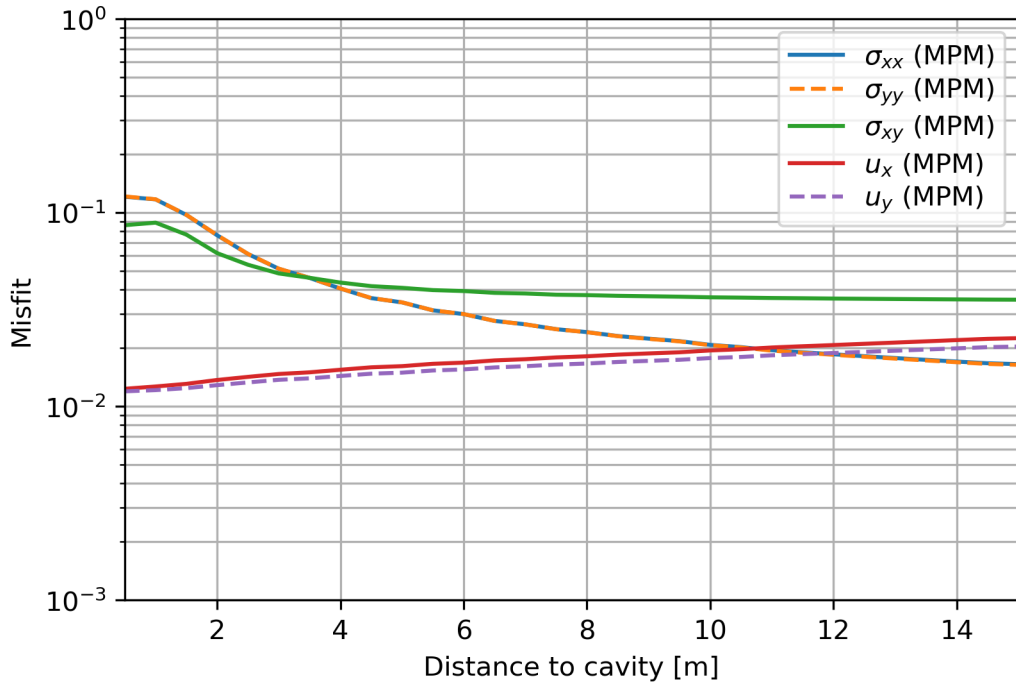

Figure 12: Case 4 misfits.

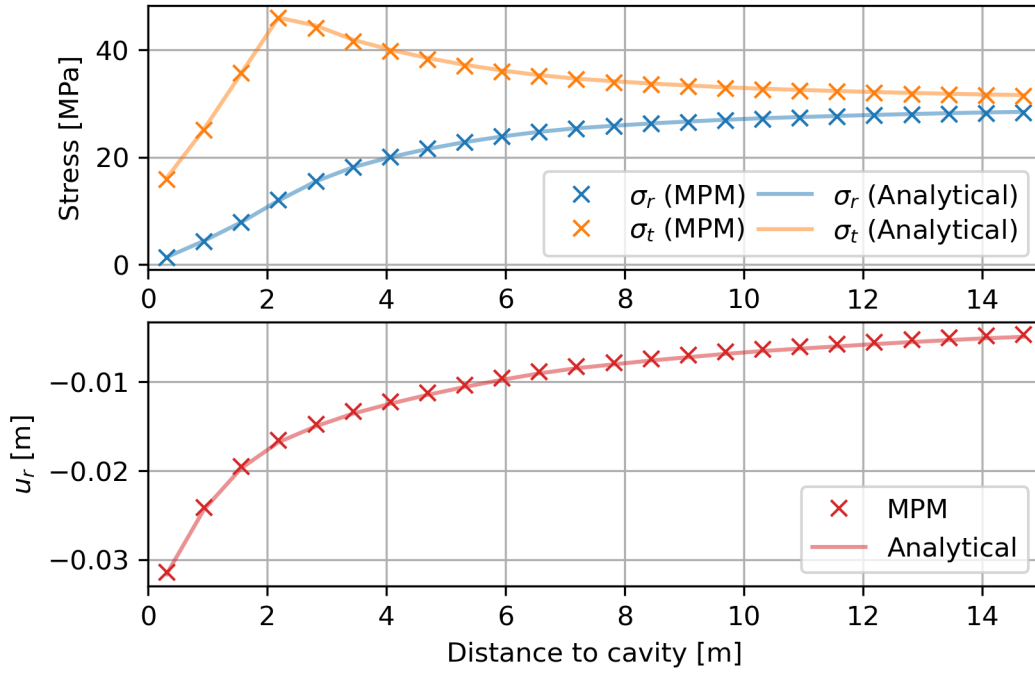

Figure 13: Case 4 radial stresses and displacements.

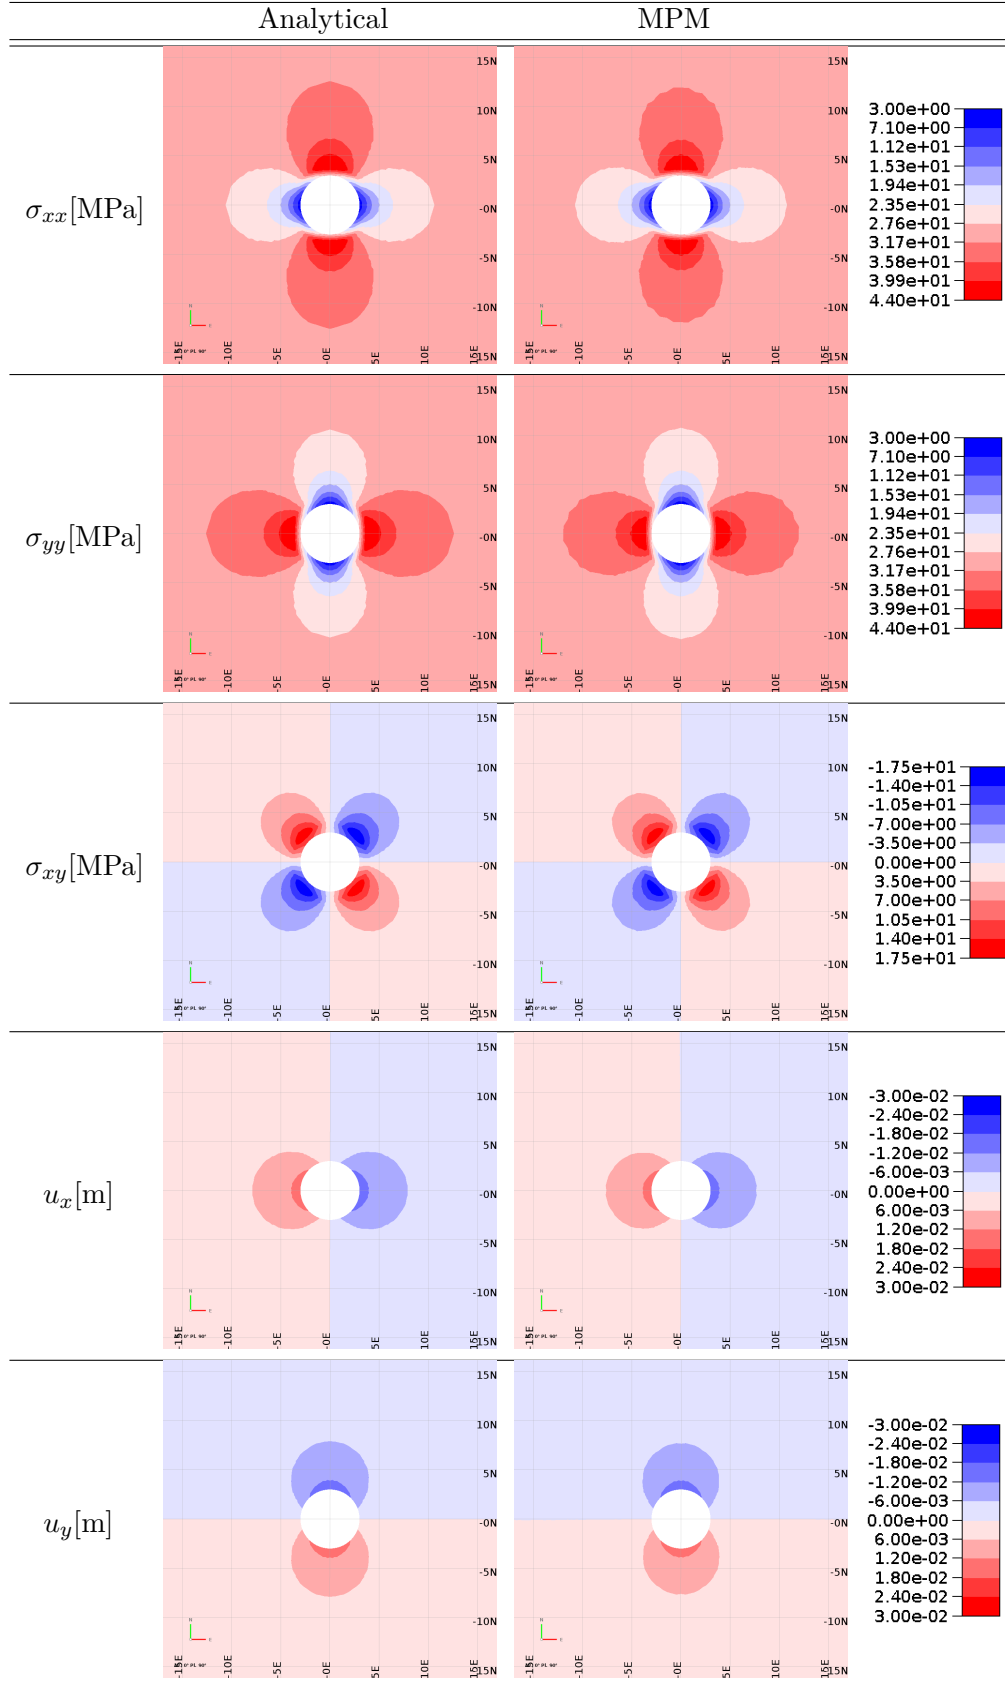

Figure 14: Case 5 stresses and displacements.

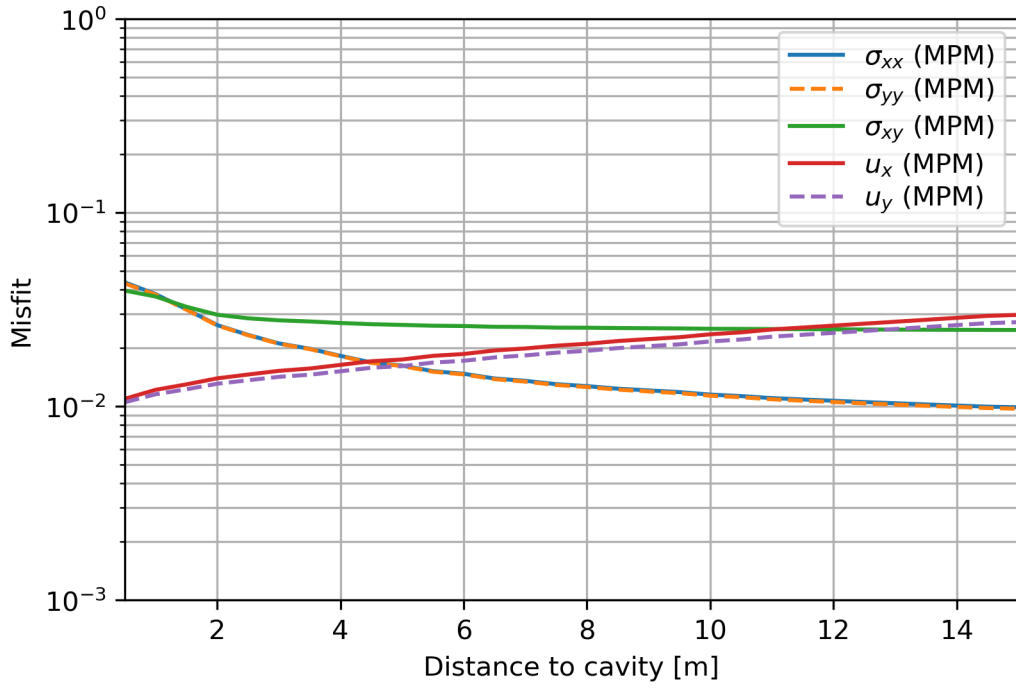

Figure 15: Case 5 misfits.

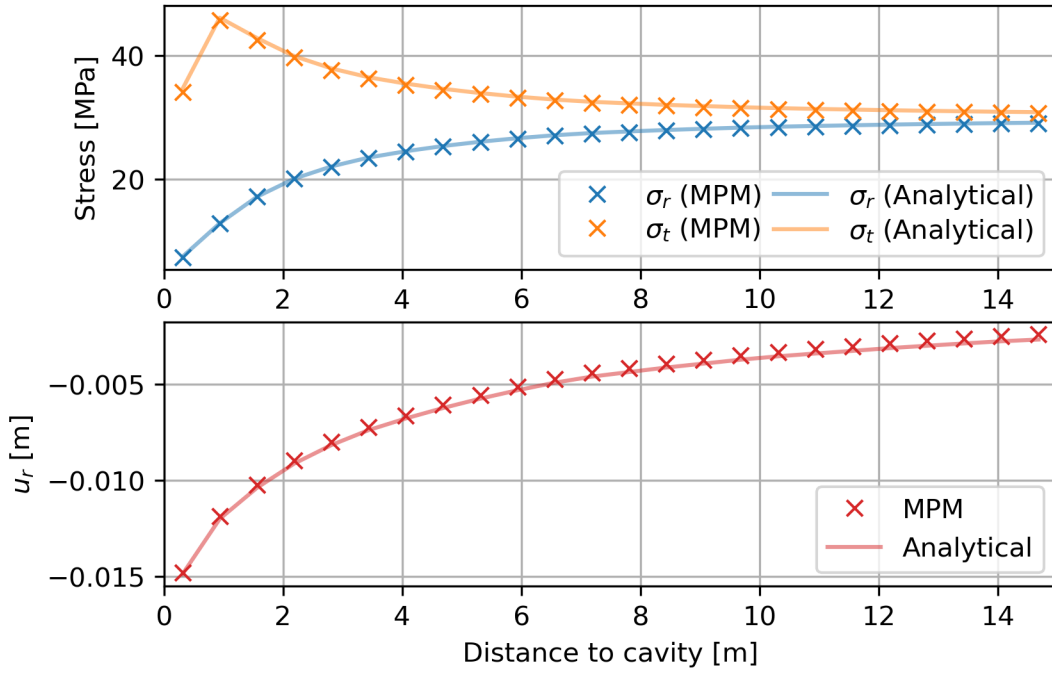

Figure 16: Case 5 radial stresses and displacements.

## 4 Hoek-Brown, cylindrical cavity [3]

Ref. [3] provides analytical solutions for a Hoek-Brown material with the same geometry and loading as described in Sec. 3.

We have again take the diameter of the cylinder to be 3 m. The surrounding material has a shear modulus of  $G = 2.8$  GPa, bulk modulus of  $K = 3.9$  GPa ( $E = 55.0$  GPa,  $\nu = 0.250$ ), density of  $\rho = 2000$  kgm<sup>-3</sup>, and Hoek-Brown parameters of  $m_b = 1.7$ ,  $s = 0.0039$ ,  $a = 0.5$ , and  $\sigma_{ci} = 30$  MPa. Both associated and non-associated flow rules are considered.

The only difference in the MPM setup to that described in Sec. 3 is the further reduction to 50 points around the cavity's circumference.

### 4.1 Case 6 - non-associated

In the first case considered, a non-associated flow rule is used. Contour plots comparing the solutions are given in Fig. 17, misfits are given in Fig. 18, and radial plots are given in Fig. 19.

### 4.2 Case 7 - associated

In the second case considered, an associated flow rule is used. Contour plots comparing the solutions are given in Fig. 20. Note that the solutions marked “analytical” in this case are not strictly analytical as they require numerically solving the ODE outlined in Appendix A.5 of Ref. [3], misfits are given in Fig. 21, and radial plots are given in Fig. 22.

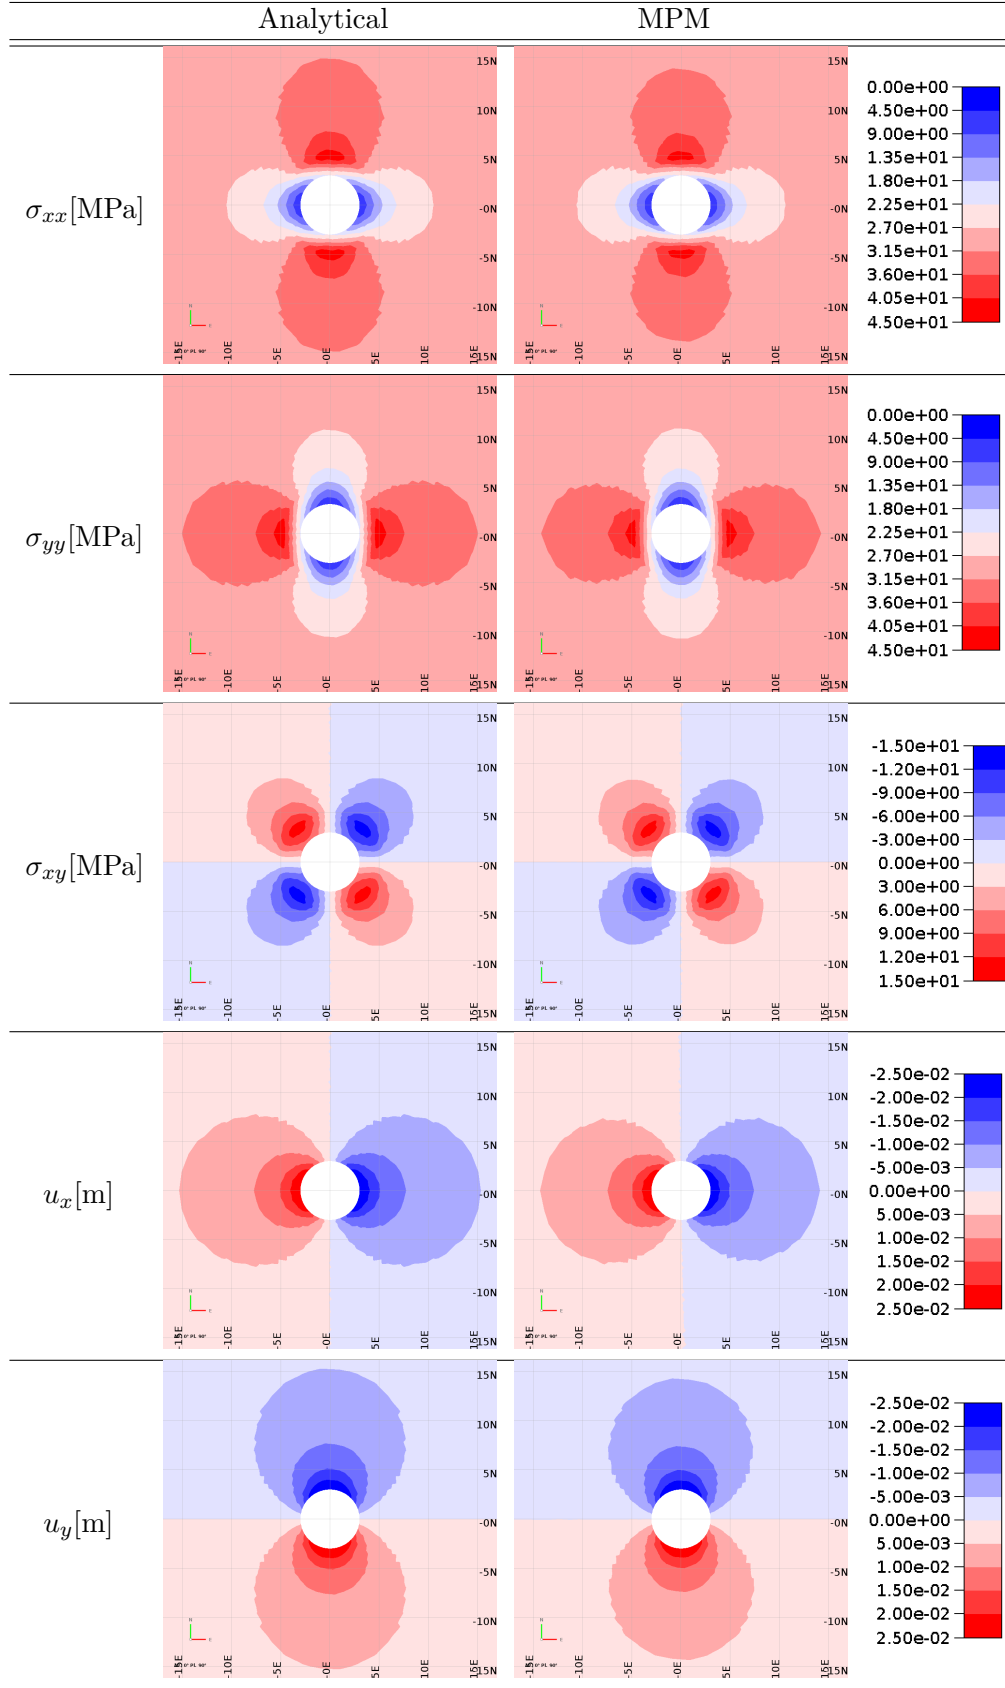

Figure 17: Case 6 stresses and displacements.

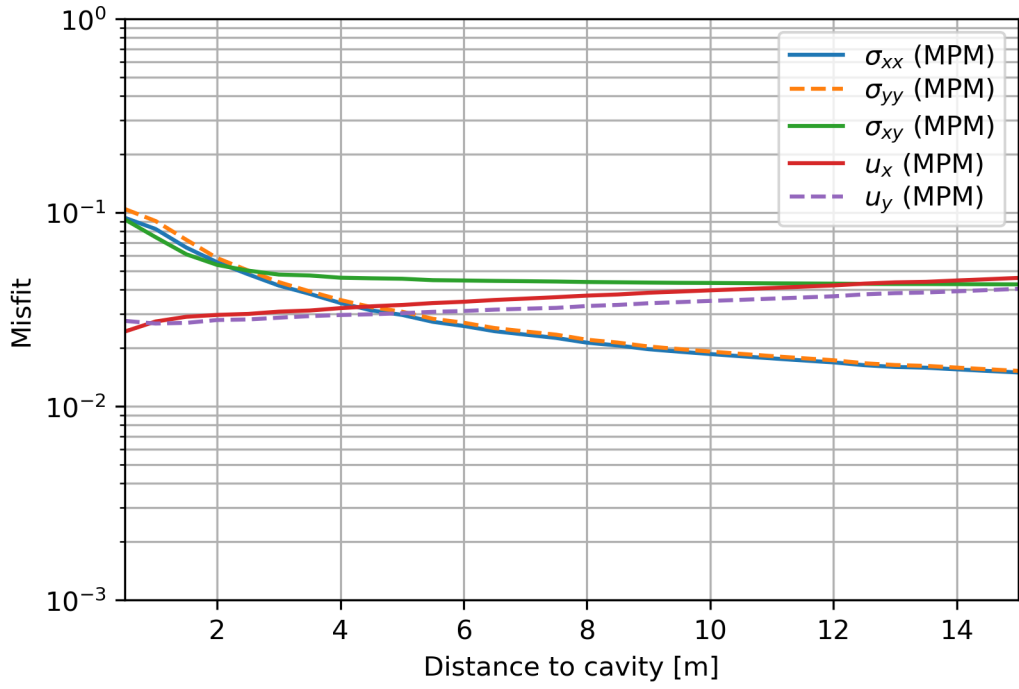

Figure 18: Case 6 misfits.

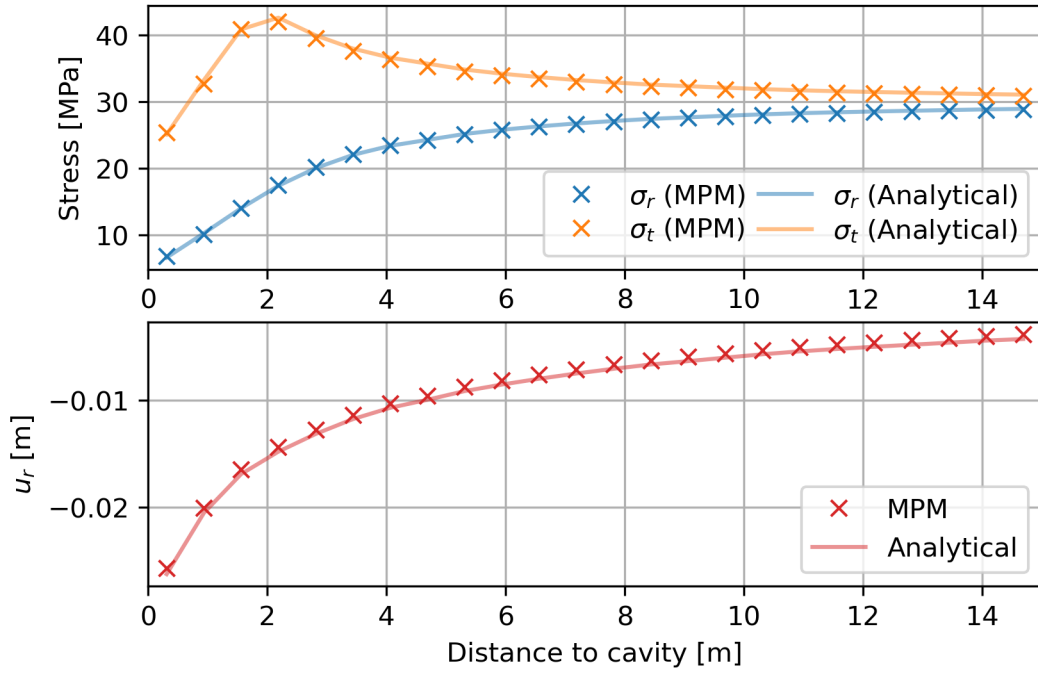

Figure 19: Case 6 radial stresses and displacements.

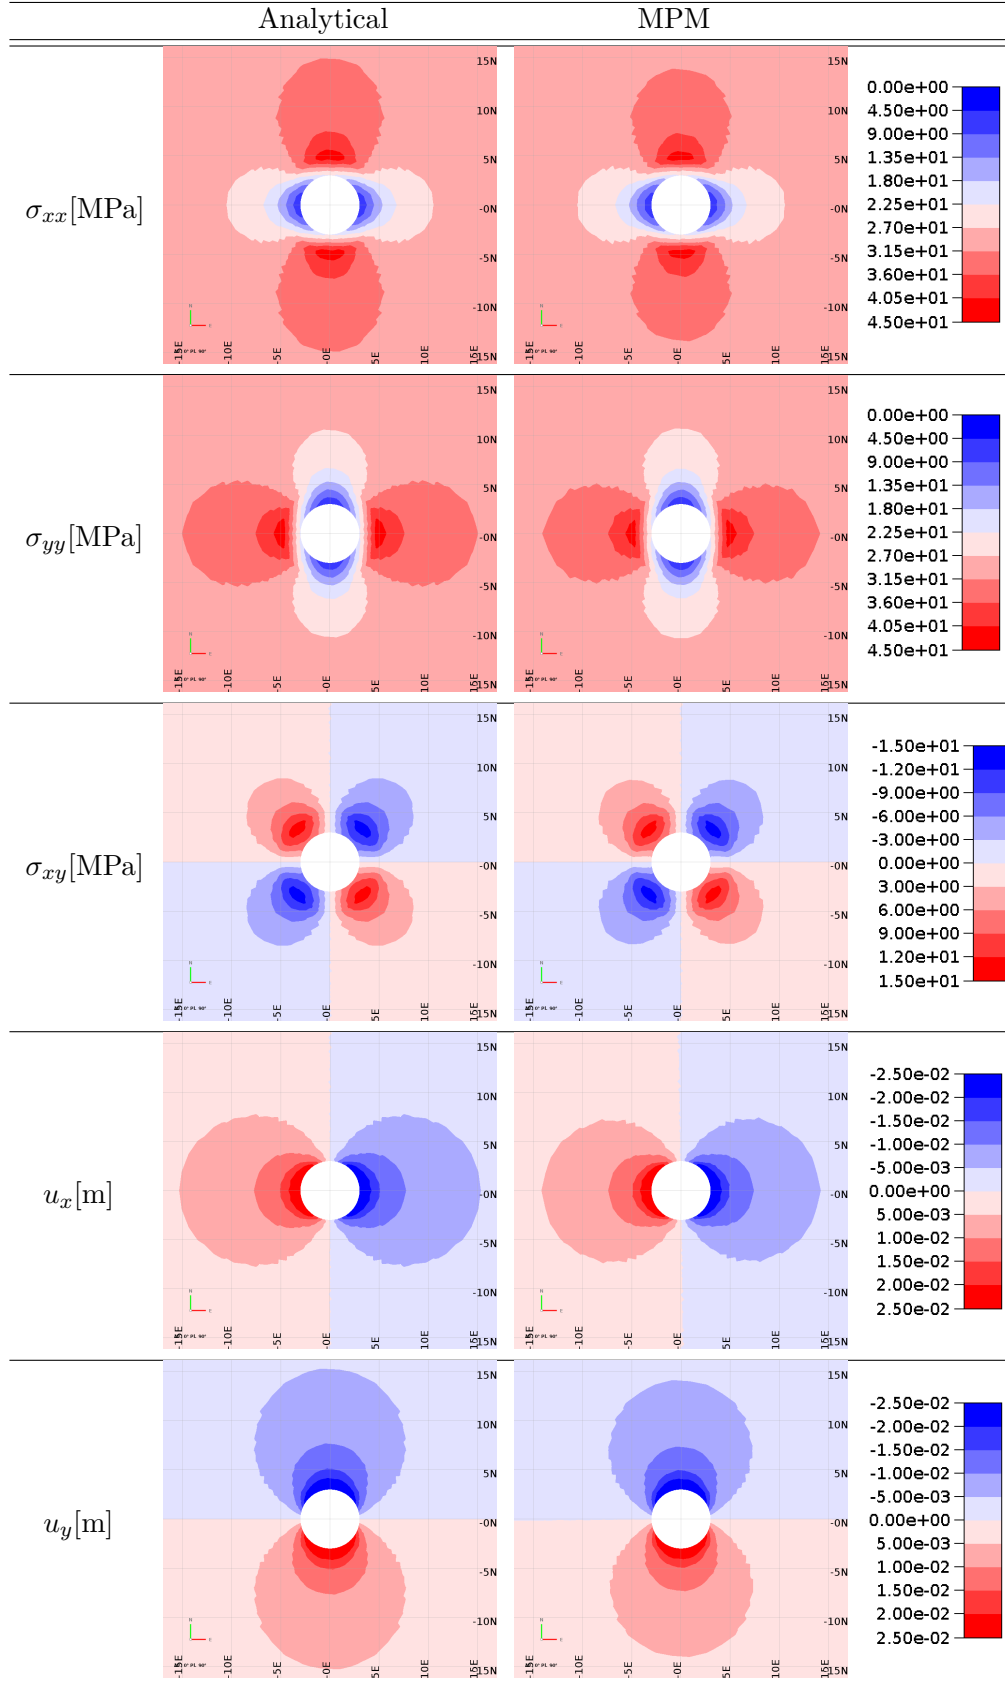

Figure 20: Case 7 stresses and displacements.

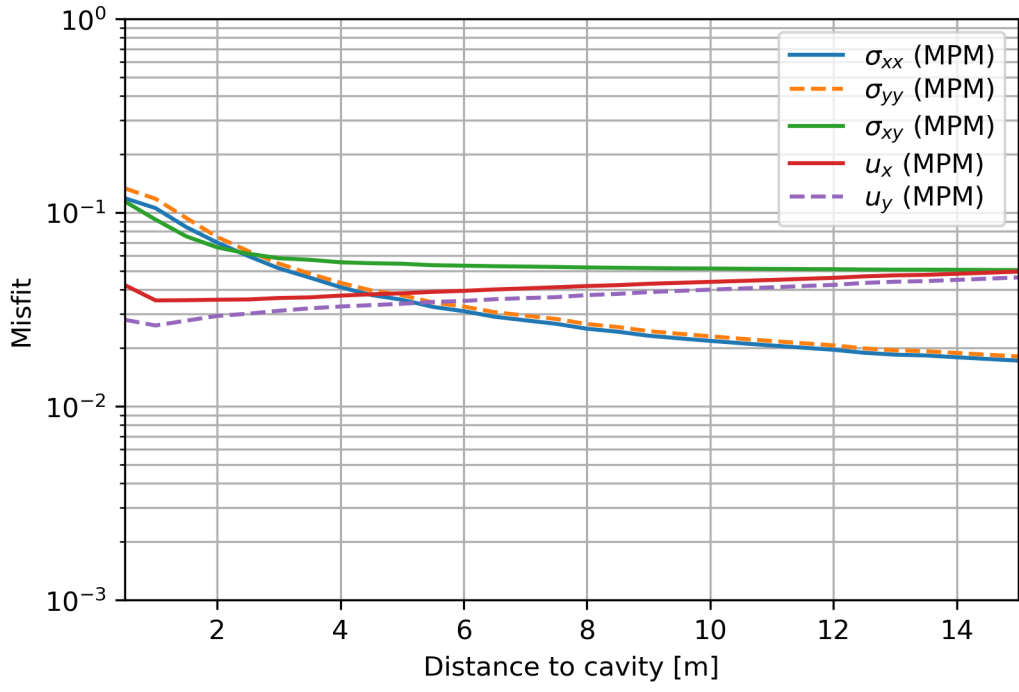

Figure 21: Case 7 misfits.

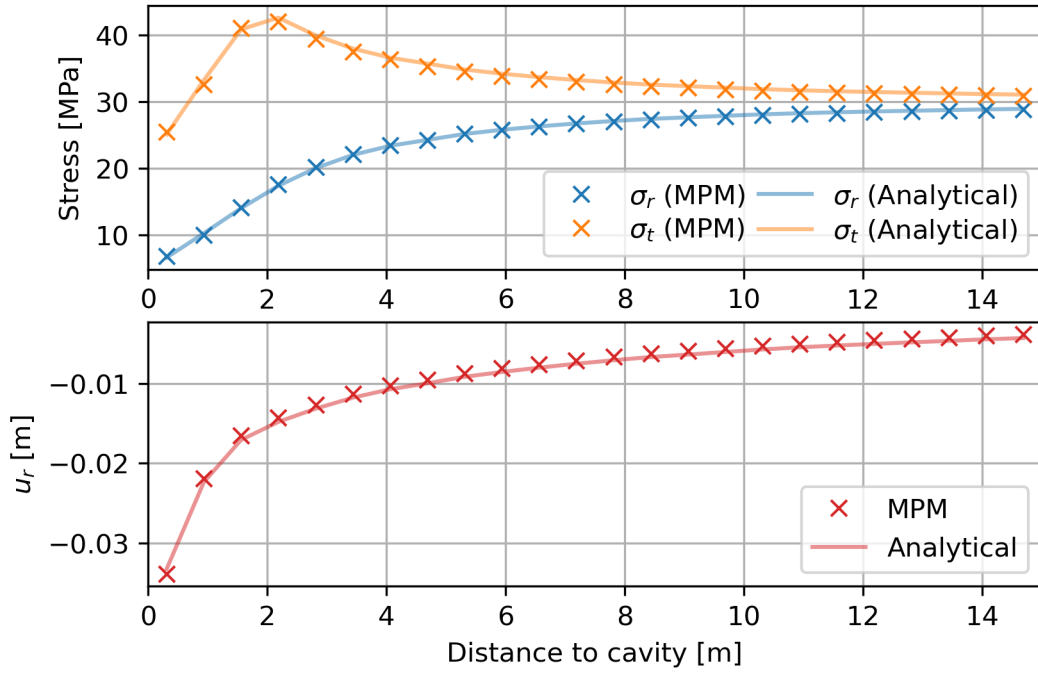

Figure 22: Case 7 radial stresses and displacements.

## References

- [1] D. Maugis. Stresses and displacements around cracks and elliptical cavities: Exact solutions. *Engineering Fracture Mechanics*, 43:217–255, 1992.
- [2] J Salencon. Contraction quasi-statique d’une cavité à symétrie sphérique ou cylindrique dans un milieu elastoplastique. In *Annales des ponts et chaussées*, volume 4, pages 231–236, 1969.
- [3] Carlos Carranza-Torres and C Fairhurst. The elasto-plastic response of underground excavations in rock masses that satisfy the Hoek–Brown failure criterion. *International Journal of Rock Mechanics and Mining Sciences*, 36(6):777–809, 1999.
